# Supplementary material for: Natural Language Robot Programming: NLP integrated with autonomous robotic grasping
Source: arXiv:2304.02993 source file (2023-04-06)
Supplement: Supplementary file 1 [file appendix.tex]

\section{Appendix}
This is appendix
